# Supplementary material for: Quantum Spontaneous Stochasticity
Source: arXiv:1509.04941 ancillary file (2015-09-16)
Supplement: Supplementary file 1 [file MathCompMethods.pdf]

# Mathematical and Computational Methods

## CONTENTS

|                                                      |    |
|------------------------------------------------------|----|
| I. Mathematical formulae for the Kummer potential    | 1  |
| A. Derivation by convolution with a Gaussian         | 1  |
| B. Derivatives of the Kummer potential               | 2  |
| C. Plots of the Kummer, spliced, and cusp potentials | 2  |
| II. Analytical results for the cusp potential        | 3  |
| A. Derivation of Eq. (11)                            | 3  |
| B. Formula for $J_t(x_0)$                            | 3  |
| C. Formula for $-J'_t(x_0)/J_t(x_0)$                 | 4  |
| III. Analytical results for the spliced potential    | 4  |
| A. Formula for $J_t(x_0)$                            | 4  |
| B. Formula for $-J'_t(x_0)/J_t(x_0)$                 | 6  |
| IV. WKB approximation                                | 6  |
| A. Mathematical framework                            | 6  |
| 1. Time-integration of the wave-function             | 6  |
| 2. Bifurcation analysis for splitting-time           | 7  |
| B. Numerical WKB methods                             | 8  |
| 1. Time-integration of the wave-function             | 8  |
| 2. Additional figures generated by the code          | 9  |
| 3. Bifurcation analysis for splitting-time           | 9  |
| V. Numerical Schrödinger methods                     | 11 |
| References                                           | 11 |

## I. MATHEMATICAL FORMULAE FOR THE KUMMER POTENTIAL

### A. Derivation by convolution with a Gaussian

Here we derive the analytical form for the Kummer potential (12) which appears in the text, as a special case of a general result for any space dimension  $d$ . This involves convolving a power-law with a Gaussian filter kernel:

$$\overline{(|\mathbf{x}|^\alpha)_\ell} \equiv \frac{1}{(2\pi)^{d/2}\ell^d} \int_{R^d} |\mathbf{x}'|^\alpha e^{-|\mathbf{x}'-\mathbf{x}|^2/2\ell^2} d^d x'.$$

This integral can be evaluated in hyperspherical coordinates for  $\mathbf{x}'$  with the angle  $\theta'_1 \equiv \theta'$  angle measured relative to  $\mathbf{x}$  and by integrating out the remaining  $(d-1)$  angles, which yields

$$\overline{(|\mathbf{x}|^\alpha)_\ell} = \frac{S_{d-1}}{(2\pi)^{d/2}\ell^d} e^{-r^2/2\ell^2} \int_0^\infty r'^{d+\alpha-1} dr' \int_0^\pi d\theta' e^{-r'^2/2\ell^2} e^{rr' \cos \theta' / \ell^2} \sin^{d-2} \theta',$$

where  $r = |\mathbf{x}|$ ,  $r' = |\mathbf{x}'|$ , and  $S_{d-1} = 2\pi^{(d-1)/2}\Gamma(\frac{d-1}{2})$  is the hypersurface area of a unit sphere in the  $(d-1)$ -dimensional space which has been integrated out. Introducing  $\rho = r/\ell$ ,  $\rho' = r'/\ell$  one finds

$$\overline{(|\mathbf{x}|^\alpha)_\ell} = \frac{\ell^\alpha}{\sqrt{\pi} 2^{\frac{d}{2}-1} \Gamma(\frac{d-1}{2})} e^{-\rho^2/2} \int_0^\infty d\rho' e^{-\rho'^2/2} \rho'^{d+\alpha-1} \int_0^\pi d\theta' e^{\rho\rho' \cos \theta'} \sin^{d-2} \theta'. \quad (\text{S1})$$

We identify in the previous expression the modified Bessel function [AS, 9.6.18]:

$$I_\nu(z) = \frac{(z/2)^\nu}{\sqrt{\pi}\Gamma(\nu + \frac{1}{2})} \int_0^\pi d\theta' e^{\pm z \cos \theta'} \sin^{2\nu} \theta'.$$

Choosing  $\nu = d/2 - 1$ , and  $z = \rho\rho'$ , we rewrite the expression (S1):

$$\overline{(|\mathbf{x}|^\alpha)_\ell} = \frac{\ell^\alpha e^{-\rho^2/2}}{\rho^{\frac{d}{2}-1}} \int_0^\infty \rho' d\rho' e^{-\rho'^2/2} \rho'^{\frac{d}{2}+\alpha-1} I_{\frac{d}{2}-1}(\rho\rho')$$

Introducing new coordinates  $t = \frac{1}{2}\rho'^2$  so that  $dt = \rho' d\rho'$  and  $\beta = \rho^2/2$ , we have

$$\begin{aligned} \overline{(|\mathbf{x}|^\alpha)_\ell} &= \frac{\ell^\alpha e^{-\rho^2/2}}{\rho^{\frac{d}{2}-1}} 2^{\mu-1} \int_0^\infty dt e^{-t} (2t)^{\mu-1} I_{2\nu}(2\beta^{1/2} t^{1/2}) \\ &= \frac{\ell^\alpha e^{-\rho^2/2}}{\rho^{\frac{d}{2}-1}} 2^{\mu-1} \frac{\Gamma(\mu+\nu)\beta^\nu}{\Gamma(2\nu+1)} {}_1F_1(\mu+\nu, 2\nu+1; \beta) \end{aligned}$$

with  $\mu = \frac{1}{2}(\frac{d}{2} + \alpha + 1)$  and  $\nu = \frac{1}{2}(\frac{d}{2} - 1)$ . The second equality above uses [BE, 4.14 (35)]:

$$\int_0^\infty dt e^{-t} (2t)^{\mu-1} J_{2\nu}(2\beta^{1/2} t^{1/2}) = \frac{\Gamma(\mu+\nu)\beta^\nu}{\Gamma(2\nu+1)} {}_1F_1(\mu+\nu, 2\nu+1; -\beta)$$

by sending  $\beta \rightarrow -\beta$  and noting that  $J_{2\nu}(iz) = i^{2\nu} I_{2\nu}(z)$  for  $-\pi < \arg z \leq \pi/2$ . Substituting back for  $\mu$ ,  $\nu$  and  $\beta$  and applying a Kummer transformation  $e^{-z} {}_1F_1(a, b; z) = {}_1F_1(b-a, b; -z)$  [EB, 6.3.7] gives our final result:

$$\overline{(|\mathbf{x}|^\alpha)_\ell} = \ell^\alpha 2^{\alpha/2} \frac{\Gamma(\frac{d+\alpha}{2})}{\Gamma(\frac{d}{2})} {}_1F_1(-\frac{\alpha}{2}, \frac{d}{2}; -\frac{|\mathbf{x}|^2}{2\ell^2}).$$

The formula for the Kummer potential (setting  $d = 1$  and sending  $\alpha \rightarrow 1 + \alpha$ ) follows immediately:

$$V_\ell(x) = -\frac{C}{1+\alpha} \overline{(|x|^{1+\alpha})_\ell} = -C\ell^{1+\alpha} \frac{2^{(1+\alpha)/2} \Gamma((2+\alpha)/2)}{(1+\alpha)\sqrt{\pi}} {}_1F_1\left(-\frac{1}{2}(1+\alpha), \frac{1}{2}; -\frac{x^2}{2\ell^2}\right). \quad (\text{S2})$$

### B. Derivatives of the Kummer potential

In estimating splitting times, we use convenient formulas for the derivatives of the potential. These are derived here. Using the elementary formula [EB, 6.4.8; AS, 13.4.8]:

$$\frac{d}{dz} {}_1F_1(a, b; z) = \frac{a}{b} {}_1F_1(a+1, b+1; z),$$

we get easily

$$V'_\ell(x) = -Cx\ell^{\alpha-1} \frac{2^{(1+\alpha)/2}\Gamma((2+\alpha)/2)}{\sqrt{\pi}} {}_1F_1\left(\frac{1}{2}(1-\alpha), \frac{3}{2}; -\frac{x^2}{2\ell^2}\right) \quad (\text{S3})$$

Introducing  $z = -x^2/2\ell^2$ , the second derivative is then:

$$V''_\ell(x) = -C\ell^{\alpha-1} \frac{2^{(1+\alpha)/2}\Gamma((2+\alpha)/2)}{\sqrt{\pi}} \left[ {}_1F_1\left(\frac{1}{2}(1-\alpha), \frac{3}{2}; z\right) + 2z \frac{d}{dz} {}_1F_1\left(\frac{1}{2}(1-\alpha), \frac{3}{2}; z\right) \right].$$

The recurrence relation [EB, 6.4.9; AS, 13.4.13]

$$z \frac{d}{dz} {}_1F_1(a, b; z) + (b-1) {}_1F_1(a, b; z) = (b-1) {}_1F_1(a, b-1; z),$$

for  $a = (1-\alpha)/2$ ,  $b = 3/2$  then yields the result quoted in the main text:

$$V''_\ell(x) = -C\ell^{\alpha-1} \frac{2^{(1+\alpha)/2}\Gamma((2+\alpha)/2)}{\sqrt{\pi}} {}_1F_1\left(\frac{1}{2}(1-\alpha), \frac{1}{2}; -\frac{x^2}{2\ell^2}\right). \quad (\text{S4})$$

Using (S4), the third derivative for the Kummer potential is computed in the same way as the first:

$$V'''_\ell(x) = -(1-\alpha)Cx\ell^{\alpha-3} \frac{2^{(1+\alpha)/2}\Gamma((2+\alpha)/2)}{\sqrt{\pi}} {}_1F_1\left(\frac{1}{2}(3-\alpha), \frac{3}{2}; -\frac{x^2}{2\ell^2}\right). \quad (\text{S5})$$

### C. Plots of the Kummer, spliced, and cusp potentials

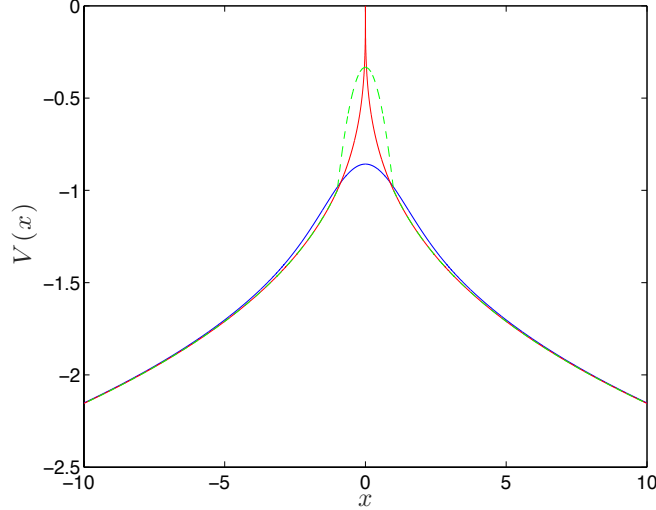

FIG. 1. Plots of the Kummer potential (blue solid), the spliced potential (green dashed), and cusp potential (red solid). Here the roughness exponent  $\alpha = 1/3$  and the UV-cutoff length  $\ell = 1$ .

## II. ANALYTICAL RESULTS FOR THE CUSP POTENTIAL

### A. Derivation of Eq. (11)

We begin with the case  $H_0 < 0$ , with  $\bar{x}_0$  introduced by  $H_0 = -\frac{C}{1+\alpha}|\bar{x}_0|^{1+\alpha}$ . Separating variables in Eq. (10) gives

$$\pm \left( \frac{2C}{1+\alpha} \right)^{1/2} (t - t_0) = \int_{x_0}^x \frac{d\xi}{\sqrt{\xi^{\alpha+1} - \bar{x}_0^{\alpha+1}}} = \frac{\bar{x}_0^{(1-\alpha)/2}}{(1+\alpha)} \int_{(x_0/\bar{x}_0)^{1+\alpha}}^{(x/\bar{x}_0)^{\alpha+1}} \frac{du}{u^{\frac{3\alpha+1}{2(\alpha+1)}}} \left( 1 - \frac{1}{u} \right)^{-1/2}, \quad (\text{S6})$$

where we have made the change of variables  $u = (\xi/\bar{x}_0)^{1+\alpha}$  to obtain the second equality. By its definition  $|\bar{x}_0| < |x_0|$ , implying  $u > 1$  strictly and absolute convergence of the standard binomial series

$$\left( 1 - \frac{1}{u} \right)^{-1/2} = \sum_{k=0}^{\infty} \frac{\left( \frac{1}{2} \right)_k}{k!} \left( -\frac{1}{u} \right)^k,$$

with the rising factorial (Pochhammer symbol)  $(a)_k = a(a+1)\cdots(a+k-1)$ . Termwise integration gives

$$\begin{aligned} \int \frac{du}{u^{\frac{3\alpha+1}{2(\alpha+1)}}} \left( 1 - \frac{1}{u} \right)^{-1/2} &= \frac{2(1+\alpha)}{1-\alpha} u^{\frac{1-\alpha}{2(1+\alpha)}} \sum_{k=0}^{\infty} \frac{\left( -\frac{1}{2} \right)_k \left( \frac{\alpha-1}{2(\alpha+1)} \right)_k}{k! \left( \frac{3\alpha+1}{2(\alpha+1)} \right)_k} \left( \frac{1}{u} \right)^k \\ &= \frac{2(1+\alpha)}{1-\alpha} u^{\frac{1-\alpha}{2(1+\alpha)}} {}_2F_1 \left( \frac{1}{2}, -\frac{(1-\alpha)}{2(1+\alpha)}; \frac{1+3\alpha}{2(1+\alpha)}; +\frac{1}{u} \right) \end{aligned}$$

where we have used the standard series definition of the hypergeometric function [EB, 2.1.1(2); AS 15.1.1] and now the symbol  $(a)_k$  represents (perhaps confusingly, but universally in the hypergeometric function literature) the falling factorial  $(a)_k \equiv a(a-1)\cdots(a-k+1)$ . Substituting this result back into (S6) gives Eq. (11) in the main text.

The case  $H_0 > 0$  is almost identical, with  $\bar{x}_0$  now introduced by  $H_0 = \frac{C}{1+\alpha}|\bar{x}_0|^{1+\alpha}$  but with otherwise the same substitution in the integral and the same series expansion, noting now that

$$\int \frac{du}{u^{\frac{3\alpha+1}{2(\alpha+1)}}} \left( 1 + \frac{1}{u} \right)^{-1/2} = \frac{2(1+\alpha)}{1-\alpha} u^{\frac{1-\alpha}{2(1+\alpha)}} {}_2F_1 \left( \frac{1}{2}, -\frac{(1-\alpha)}{2(1+\alpha)}; \frac{1+3\alpha}{2(1+\alpha)}; -\frac{1}{u} \right).$$

### B. Formula for $J_t(x_0)$

Since the definition of  $x_t(x_0)$  assumes  $p_0 = 0$ , thus  $\bar{x}_0 = x_0$  and we have the following relation:

$$\left( \frac{x_t}{x_0} \right)^{(1-\alpha)/2} {}_2F_1 \left( \frac{1}{2}, -\frac{(1-\alpha)}{2(1+\alpha)}; \frac{1+3\alpha}{2(1+\alpha)}; +\left( \frac{x_0}{x_t} \right)^{1+\alpha} \right) - {}_2F_1 \left( \frac{1}{2}, -\frac{(1-\alpha)}{2(1+\alpha)}; \frac{1+3\alpha}{2(1+\alpha)}; +1 \right) = \left( \frac{x_+(t)}{x_0} \right)^{(1-\alpha)/2}.$$

We have assumed for simplicity that  $x_0 > 0$ ; otherwise, if  $x_0 < 0$ , replace  $x_+(t)$  by  $x_-(t)$ . We differentiate both sides with respect to  $x_0$ , applying the identity [AS 15.2.3]

$$\frac{d}{dz} [z^b {}_2F_1(a, b; c; z)] = bz^{b-1} {}_2F_1(a, b+1; c; z),$$

with  $z = (x_0/x_t)^{1+\alpha}$  and

$$\frac{dz}{dx_0} = (1+\alpha) \left[ \frac{x_0^\alpha}{x_t^{1+\alpha}} - \frac{x_0^{1+\alpha}}{x_t^{2+\alpha}} J_t(x_0) \right].$$

We arrive at the equation:

$$-\frac{(1-\alpha)}{2} \left( \frac{x_t}{x_0} \right)^{\frac{3+\alpha}{2}} {}_2F_1 \left( \frac{1}{2}, \frac{1+3\alpha}{2(1+\alpha)}; \frac{1+3\alpha}{2(1+\alpha)}; +\left( \frac{x_0}{x_t} \right)^{1+\alpha} \right) \frac{x_0^\alpha}{x_t^{1+\alpha}} \left[ 1 - \frac{x_0}{x_t} J_t(x_0) \right] = -\frac{(1-\alpha)}{2x_0} \left( \frac{x_+(t)}{x_0} \right)^{(1-\alpha)/2}.$$

Solving yields

$$J_t = \frac{x_t}{x_0} \left[ 1 - \frac{1}{F} \left( \frac{x_+}{x_t} \right)^{(1-\alpha)/2} \right],$$

where  $F$  stands for the hypergeometric function in the formula above, which can be evaluated with the identity [AS.15.1.8]:

$${}_2F_1(a, b; b; z) = (1 - z)^{-a}.$$

Simplifying the resultant expression yields

$$J_t(x_0) = \frac{1}{x_0} \left[ x_t - (x_+(t))^{(1-\alpha)/2} \sqrt{x_t^{1+\alpha} - x_0^{1+\alpha}} \right].$$

which is the result in the main text.

For  $t \gg t_0$ ,  $x_t \sim x_+(t) \gg x_0$ . According to this result, the leading contribution to  $J_t$  cancels at long times. To evaluate asymptotics of  $J_t$  one needs a more accurate formula that follows from the first equation in this section:

$$\begin{aligned} x_t &\sim x_+(t) \left[ 1 + F(1) \left( \frac{x_0}{x_+(t)} \right)^{(1-\alpha)/2} \right]^{2/(1-\alpha)} \\ &\sim x_+(t) + \frac{2}{1-\alpha} F(1) [x_+(t)]^{(1+\alpha)/2} x_0^{(1-\alpha)/2}, \end{aligned}$$

where  $F(1) \equiv {}_2F_1\left(\frac{1}{2}, -\frac{(1-\alpha)}{2(1+\alpha)}; \frac{1+3\alpha}{2(1+\alpha)}; +1\right)$ . Substituting into the expression for  $J_t(x_0)$  one easily finds that

$$J_t(x_0) \sim F(1) \left( \frac{x_+(t)}{x_0} \right)^{(1+\alpha)/2}, \quad t \gg t_0.$$

### C. Formula for $-J'_t(x_0)/J_t(x_0)$

Direct differentiation of the exact expression for  $J_t(x_0)$  and some simplification gives

$$-J'_t(x_0)/J_t(x_0) = \frac{1+\alpha}{2} \frac{[x_+(t)]^{\frac{1-\alpha}{2}}}{x_0} \frac{x_t^\alpha - x_0^\alpha/J_t}{\sqrt{x_t^{1+\alpha} - x_0^{1+\alpha}}}.$$

Thus, for  $t \gg t_0$ ,

$$-J'_t(x_0)/J_t(x_0) \sim \frac{1+\alpha}{2} \left[ \frac{x_+(t)}{x_t} \right]^{\frac{1-\alpha}{2}} \frac{1}{x_0} \sim \frac{1+\alpha}{2} \frac{1}{x_0}.$$

## III. ANALYTICAL RESULTS FOR THE SPLICED POTENTIAL

### A. Formula for $J_t(x_0)$

For particles which are forever in the outer cusp region,  $|x_0| > \ell$ , one can use the results above for the cusp potential. For particles which start in the inner parabolic region,  $|x_0| < \ell$  one gets, trivially,

$$J_t(x_0) = \cosh \left( \frac{C^{1/2}t}{\ell^{(1-\alpha)/2}} \right), \quad t < t_\ell(x_0).$$

At times  $t > t_\ell(x_0)$ , the particle lies in the cusp region. We must then differentiate with respect to  $x_0$  the expression

$$\begin{aligned} &\left| \frac{x_t}{\bar{x}_0} \right|^{(1-\alpha)/2} {}_2F_1 \left( \frac{1}{2}, -\frac{(1-\alpha)}{2(1+\alpha)}; \frac{1+3\alpha}{2(1+\alpha)}; + \left| \frac{\bar{x}_0}{x_t} \right|^{1+\alpha} \right) - \left| \frac{\ell}{\bar{x}_0} \right|^{(1-\alpha)/2} {}_2F_1 \left( \frac{1}{2}, -\frac{(1-\alpha)}{2(1+\alpha)}; \frac{1+3\alpha}{2(1+\alpha)}; + \left| \frac{\bar{x}_0}{\ell} \right|^{1+\alpha} \right) \\ &= \frac{1}{2}(1-\alpha) \left( \frac{2C}{1+\alpha} \right)^{1/2} \bar{x}_0^{(\alpha-1)/2} (t - t_\ell(x_0)). \end{aligned}$$

which follows from (23) in the main text after dividing both sides by  $x_0^{(1-\alpha)/2}$ . The differential relation [AS 15.2.3] can now be applied to both terms on the first line. Using the definition  $J_t = \partial x_t / \partial x_0$  and the elementary results

$$\left(\frac{\bar{x}_0}{\ell}\right)^{1+\alpha} = \frac{1-\alpha}{2} + \frac{1+\alpha}{2} \left(\frac{x_0}{\ell}\right)^2, \quad \frac{\partial}{\partial x_0} \left(\frac{\bar{x}_0}{\ell}\right)^{1+\alpha} = (1+\alpha) \frac{x_0}{\ell^2}, \quad \frac{\partial \bar{x}_0}{\partial x_0} = \frac{x_0}{\bar{x}_0^\alpha \ell^{1-\alpha}},$$

$$\frac{\partial}{\partial x_0} \left(\frac{\bar{x}_0}{x_t}\right)^{1+\alpha} = (1+\alpha) \left(\frac{\bar{x}_0}{x_t}\right)^{1+\alpha} \left[ \frac{x_0}{\bar{x}_0^{1+\alpha} \ell^{1-\alpha}} - \frac{J_t(x_0)}{x_t} \right],$$

$$\frac{\partial t_\ell(x_0)}{\partial x_0} = - \left( \frac{\ell^{3-\alpha}}{C} \right)^{1/2} \frac{1}{x_0 \sqrt{\ell^2 - x_0^2}},$$

one gets after differentiation and straightforward but lengthy algebra to solve for  $J_t(x_0)$  that

$$J_t(x_0) = \frac{x_0 x_t}{\bar{x}_0^{1+\alpha} \ell^{1-\alpha}} + \frac{x^{(1+\alpha)/2}}{F(x)} \times \left[ -\frac{1}{2}(1-\alpha) \left( \frac{2C}{1+\alpha} \right)^{1/2} (t - t_\ell(x_0)) \frac{x_0}{\bar{x}_0^{1+\alpha} \ell^{1-\alpha}} + \left( \frac{2}{1+\alpha} \right)^{1/2} \ell^{(1-\alpha)/2} \frac{\ell}{x_0 \sqrt{\ell^2 - x_0^2}} - F(\ell) \frac{x_0}{\bar{x}_0^{1+\alpha} \ell^{(1-\alpha)/2}} \right].$$

where we have used the shorthand notation

$$F(x) \equiv {}_2F_1 \left( \frac{1}{2}, \frac{1+3\alpha}{2(1+\alpha)}; \frac{1+3\alpha}{2(1+\alpha)}; \left( \frac{\bar{x}_0}{x} \right)^{1+\alpha} \right).$$

Using again the identity [AS, 15.1.8] for this hypergeometric function, the result cited in the main text is obtained:

$$J_t(x_0) = \frac{x_0 x_t}{\bar{x}_0^{1+\alpha} \ell^{1-\alpha}} + \sqrt{x_t^{1+\alpha} - \bar{x}_0^{1+\alpha}} \times \left[ -\frac{1}{2}(1-\alpha) \left( \frac{2C}{1+\alpha} \right)^{1/2} (t - t_\ell(x_0)) \frac{x_0}{\bar{x}_0^{1+\alpha} \ell^{1-\alpha}} + \frac{1}{2}(1-\alpha) \left( \frac{2}{1+\alpha} \right)^{1/2} \frac{\ell^{(1+\alpha)/2} \sqrt{\ell^2 - x_0^2}}{x_0 \bar{x}_0^{1+\alpha}} \right].$$

It is worth noting that there is a finite jump-discontinuity at  $|x_0| = \ell$  between the above result for  $J_t(x_0)$  when  $|x_0| < \ell$  and the pure cusp result of the previous section when  $|x_0| > \ell$ . This accounts for the discontinuity in the WKB position probability density  $\rho_t = \rho_0/J_t$  that we see numerically for the spliced-potential model.

We now consider the asymptotics of  $J_t(x_0)$  for  $t \gg t_\ell(x_0)$ . Because

$$\frac{1}{2}(1-\alpha) \left( \frac{2C}{1+\alpha} \right)^{1/2} (t - t_\ell(x_0)) \sim [x_+(t)]^{(1+\alpha)/2}, \quad t \gg t_\ell(x_0)$$

we that there is cancellation of the leading order terms  $\propto x_+(t)$  as  $t \rightarrow \infty$ , just as for the cusp potential. The surviving terms of order  $\sim [x_+(t)]^{(1+\alpha)/2}$  arise from two sources. First there are contributions of that size from  $x_t^{(1+\alpha)/2}$  times the  $O(1)$  terms inside the large square-bracket factor of  $J_t(x_0)$ . This leads to

$$J_t(x_0) \sim \frac{x_0}{\bar{x}_0^{1+\alpha} \ell^{1-\alpha}} \left[ x_t - x_t^{(1+\alpha)/2} (x_+(t))^{(1-\alpha)/2} \right] + \left( \frac{x_t}{\ell} \right)^{(1+\alpha)/2} \Delta_1 \left( \frac{x_0}{\ell} \right) \frac{x_0 \ell^\alpha}{\bar{x}_0^{1+\alpha}}, \quad t \gg t_\ell(x_0)$$

with

$$\Delta_1 \left( \frac{x_0}{\ell} \right) = \frac{1}{2}(1-\alpha) \left( \frac{2C}{1+\alpha} \right)^{1/2} \operatorname{arccosh} \left( \frac{\ell}{x_0} \right) + \frac{1}{2}(1-\alpha) \left( \frac{2}{1+\alpha} \right)^{1/2} \frac{\ell \sqrt{\ell^2 - x_0^2}}{x_0^2}.$$

The other contributions arise from the sub-leading asymptotics of  $x_t$ . It is not hard to see from (23) in the main text [or the first equation in this section] that

$$x_t \sim \left[ (x_+(t))^{(1-\alpha)/2} + F(1) \ell^{(1-\alpha)/2} \Delta_2 \left( \frac{x_0}{\ell} \right) \right]^{2/(1-\alpha)}$$

$$\sim x_+(t) + \frac{2}{1-\alpha} (x_+(t))^{(1+\alpha)/2} \ell^{(1-\alpha)/2} \Delta_2 \left( \frac{x_0}{\ell} \right),$$

with

$$\Delta_2 \left( \frac{x_0}{\ell} \right) = {}_2F_1 \left( \frac{1}{2}, -\frac{(1-\alpha)}{2(1+\alpha)}; \frac{1+3\alpha}{2(1+\alpha)}; \left( \frac{\bar{x}_0}{\ell} \right)^{1+\alpha} \right) - \frac{1}{2}(1-\alpha) \left( \frac{2C}{1+\alpha} \right)^{1/2} \operatorname{arccosh} \left( \frac{\ell}{x_0} \right).$$

Substituting this result for  $x_t$  into the previous expression for  $J_t(x_0)$  yields the final result

$$J_t(x_0) \sim \left( \frac{x_t}{\ell} \right)^{(1+\alpha)/2} \Delta \left( \frac{x_0}{\ell} \right) \frac{x_0 \ell^\alpha}{\bar{x}_0^{1+\alpha}}$$

with

$$\Delta \left( \frac{x_0}{\ell} \right) = \Delta_1 \left( \frac{x_0}{\ell} \right) + \Delta_2 \left( \frac{x_0}{\ell} \right) = {}_2F_1 \left( \frac{1}{2}, -\frac{(1-\alpha)}{2(1+\alpha)}; \frac{1+3\alpha}{2(1+\alpha)}; \left( \frac{\bar{x}_0}{\ell} \right)^{1+\alpha} \right) + \frac{1}{2}(1-\alpha) \left( \frac{2}{1+\alpha} \right)^{1/2} \frac{\ell \sqrt{\ell^2 - x_0^2}}{x_0^2}.$$

We thus obtain the function  $G(u_0)$  mentioned in the text, with

$$G(u_0) = \Delta(u_0) u_0 / \bar{u}_0^{1+\alpha},$$

where in the denominator and in the argument of the hypergeometric function we use

$$\bar{u}_0^{1+\alpha} = \frac{1-\alpha}{2} + \frac{1+\alpha}{2} u_0^2 = 1 - \frac{1+\alpha}{2} (1 - u_0^2).$$

## B. Formula for $-J'_t(x_0)/J_t(x_0)$

The formula for  $|x_0| > \ell$  in the cusp region was worked out in the previous section, so that we discuss here only  $|x_0| < \ell$ . In this interval  $J'_t(x_0) \equiv 0$  for  $t < t_\ell(x_0)$ , so that we need consider only times  $t > t_\ell(x_0)$ . Using the exact result for  $J_t(x_0)$ , it follows by a lengthy but straightforward calculation that

$$\begin{aligned} -\frac{J'_t(x_0)}{J_t(x_0)} &= -\frac{1}{x_0} + \alpha \frac{x_0}{\bar{x}_0^{1+\alpha} \ell^{1-\alpha}} + \frac{1}{2}(1+\alpha) \frac{x_t^\alpha - \bar{\ell}^{1-\alpha} J_t(x_0)}{\sqrt{x_t^{1+\alpha} - \bar{x}_0^{1+\alpha}}} \left[ (x_+(t))^{(1-\alpha)/2} - \ell^{(1-\alpha)/2} \Delta_1 \left( \frac{x_0}{\ell} \right) \right] \frac{x_0}{\bar{x}_0^{1+\alpha} \ell^{1-\alpha}} \\ &\quad + (1-\alpha) \left( \frac{2}{1+\alpha} \right)^{1/2} \frac{\ell^{(7-\alpha)/2}}{x_0^3 \sqrt{\ell^2 - x_0^2}} \sqrt{x_t^{1+\alpha} - \bar{x}_0^{1+\alpha}} \frac{x_0}{J_t(x_0) \bar{x}_0^{1+\alpha} \ell^{1-\alpha}} \end{aligned}$$

Then using the known asymptotics of  $x_t, J_t$  for  $t \gg t_\ell(x_0)$ , one gets again straightforwardly

$$-\frac{J'_t(x_0)}{J_t(x_0)} \sim -\frac{1}{x_0} + \frac{1}{2}(1+3\alpha) \frac{x_0}{\bar{x}_0^{1+\alpha} \ell^{1-\alpha}} + (1-\alpha) \left( \frac{2}{1+\alpha} \right)^{1/2} \frac{\ell^3}{x_0^3 \sqrt{\ell^2 - x_0^2} \Delta(x_0/\ell)}, \quad t \gg t_\ell(x_0).$$

This is equivalent to the result cited in the main text.

## IV. WKB APPROXIMATION

### A. Mathematical framework

#### 1. Time-integration of the wave-function

One of the great technical advantages of the WKB approximation is that it reduces the integration of the Schrödinger equation in the semi-classical regime to integration of a set of ODE's. We write out these equations below:

$$\begin{aligned} \dot{x} &= p/m, & x(t_0) &= x_0 \\ \dot{p} &= -V'(x), & p(t_0) &= \langle p \rangle \\ \dot{J} &= K/m, & J(t_0) &= 1 \\ \dot{K} &= -V''(x)J, & K(t_0) &= 0 \\ \dot{S} &= \frac{p^2}{2m} - V(x), & S(t_0) &= S_0(x_0) \end{aligned} \tag{S7}$$

The first two equations are just Hamilton's equations for  $x_t(x_0)$  and  $p_t(x_0)$ , with the initial condition  $p(t_0) = \langle p \rangle$  coming from the mean momentum in the initial wave-function. The next two equations and the initial data for the two quantities  $J_t(x_0) = x'_t(x_0)$  and  $K_t(x_0) = p'_t(x_0)$  come from differentiating with the respect to  $x_0$  the equations and initial data in the first two lines. The final equation for the phase of the WKB wave-function comes from recognizing that it is the solution of the Hamilton-Jacobi equation and thus coincides with the classical action:

$$S_t(x_0) = S_0(x_0) + \int_0^t ds \left[ \frac{1}{2m} p_s^2(x_0) - V(x_s(x_0)) \right]$$

For the Gaussian minimal-uncertainty wave-packet,  $S_0(x_0) = \langle p \rangle x_0$ . Once these equations are integrated in time, the WKB position probability density  $\rho(x, t)$  is reconstructed from equation (16) in the main text,

$$\rho(x_t(x_0), t) = \rho_0(x_0) / J_t(x_0)$$

and the full WKB wavefunction from the similar relation

$$\psi(x_t(x_0), t) = \left( \frac{\rho_0(x_0)}{J_t(x_0)} \right)^{1/2} \exp(iS_t(x_0)/\hbar).$$

Of course, this approximation is only accurate when  $S_t \gg \hbar$  and the wave-function is rapidly oscillating.

We assumed above that the potential  $V(x)$  is twice continuously differentiable, but this is not true for the spliced potential. Thus, some further attention must be given to the evaluation of the WKB approximation in that case. In particular, the 2nd of Hamilton's equations for the spliced potential is

$$\dot{p} = -V'(x) = C\ell^{\alpha-1}x \cdot \theta(\ell - x) + C|x|^\alpha \text{sign}(x) \cdot \theta(x - \ell),$$

with the derivative of the potential defined piecewise. Here  $\theta(x)$  is the Heaviside step-function. Hence, the differentiation of this equation with respect to  $x_0$  could lead to additional delta-function terms. Fortunately, these cancel because of continuity of the 1st-derivative  $V'(x)$  of the spliced potential at  $x = \ell$ :

$$\dot{K} = \underbrace{[C\ell^{\alpha-1} \cdot \theta(\ell - x) + \alpha C|x|^{\alpha-1} \cdot \theta(x - \ell)]}_{-V''(x)} J + [C\ell^{\alpha-1}x - C|x|^\alpha \text{sign}(x)] J \cdot \delta(x - \ell),$$
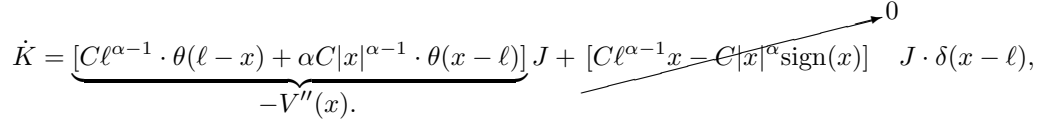

The resulting equation is the same as for the twice continuously differentiable potentials if, as indicated just above, we interpret  $V''(x)$  as the piecewise 2nd-derivative.

## 2. Bifurcation analysis for splitting-time

The bifurcation analysis followed in the main text in order to calculate wave-function splitting times requires solution of the dynamical evolution of  $J'_t(x_0) = x''_t(x_0)$ . This is most easily obtained by adjoining to the previous system of five ODE's the additional pair of equations:

$$\begin{aligned} \dot{J}' &= K', & J'(t_0) &= 0 \\ \dot{K}' &= -V''(x)J' - V'''(x)J^2, & K'(t_0) &= 0. \end{aligned} \tag{S8}$$

These are readily obtained by differentiating with respect to  $x_0$  the equations and initial conditions for  $J_t, K_t$ . Using the equations for  $J, K, J', K'$ , it is easily shown that

$$\frac{d}{dt}(K'J - J'K) = -V'''(x)J^3, \quad (K'J - J'K)(t_0) = 0.$$

For the class of potentials of interest,  $V'''(x) > 0$  for  $x > 0$  and  $V'''(x) < 0$  for  $x < 0$ . By the symmetry of the problem about  $x = 0$ , we can restrict attention just to  $x > 0$ , where it follows that  $K'J - J'K \leq 0$ . But furthermore

$$\frac{d}{dt}(-J'/J) = -(K'J - J'K)/J^2, \quad J'(t_0)/J(t_0) = 0.$$

Hence,  $\frac{d}{dt}(-J'/J) \geq 0$  for  $x > 0$ , as claimed in the main text.



This same argument applies to the spliced potential, with some slight modifications. Unlike in the equation for  $K$  discussed previously, the delta-function in the equation for  $K'$  no longer cancels, because  $V''(x)$  is not continuous at  $x = \ell$ . In fact,

$$\dot{K}' = \underbrace{[C\ell^{\alpha-1} \cdot \theta(\ell - x) + \alpha C|x|^{\alpha-1} \cdot \theta(x - \ell)]}_{-V''(x)} J' + \underbrace{\alpha(\alpha - 1)C|x|^{\alpha-2} \text{sign}(x) \cdot \theta(x - \ell) J^2 - (1 - \alpha)\ell^{\alpha-1} J^2 \cdot \delta(x - \ell)}_{-V'''(x)},$$

where  $V''(\ell+) - V''(\ell-) = -(1 - \alpha)\ell^{\alpha-1}$  and above we have defined  $V''(x)$ ,  $V'''(x)$  piecewise. Integrating the equations for  $J'$ ,  $K'$  by using  $J'_t(x_0) = K'_t(x_0) \equiv 0$  for  $t < t_\ell(x_0)$  and  $\delta(x_t(x_0) - \ell) = \delta(t - t_\ell(x_0))/|\dot{x}_t(x_0)|$  one finds that

$$\begin{aligned} J'_t(x_0) \Big|_{t=t_\ell(x_0)+} &= 0 \\ K'_t(x_0) \Big|_{t=t_\ell(x_0)+} &= -(1 - \alpha)\ell^{\alpha-1} \frac{J_t^2(x_0)}{|p_t(x_0)/m|} \Big|_{t=t_\ell(x_0)} < 0. \end{aligned}$$

Thus,

$$K'_t J_t - J'_t K_t = 0, \quad t < t_\ell(x_0).$$

but

$$(K'_t J_t - J'_t K_t) \Big|_{t=t_\ell(x_0)+} = K'_t J_t \Big|_{t=t_\ell(x_0)+} < 0,$$

where we note  $J_t > 0$ ,  $K_t > 0$  for all times  $t$ . In particular, for  $t = t_\ell(x_0)$  it is easy using the inverted oscillator dynamics in the interval  $|x| < \ell$  to show that

$$J_t(x_0) = \frac{\ell}{|x_0|}, \quad K_t(x_0) = \left( \frac{C}{\ell^{1-\alpha}} \right)^{1/2} \sqrt{\left( \frac{\ell}{x_0} \right)^2 - 1}, \quad t = t_\ell(x_0).$$

Hence  $(K'_t J_t - J'_t K_t)$  starts as negative at  $t = t_\ell(x_0)$  and this sign is preserved by the cusp dynamics for  $t > t_\ell(x_0)$ , by the same argument as for general smooth potentials. Hence, the entire argument goes through.

## B. Numerical WKB methods

### 1. Time-integration of the wave-function

The numerical results for the WKB wave-function evolution presented in the paper are carried out by numerically integrating the system of ODE's in Eq.(S7) for a grid of initial  $x_0$ -values. The integrations were carried out in Matlab, using the variable-order (1-13) solver `ode113` and imposing small error tolerances ( $10^{-8}$  relative error,  $10^{-14}$  absolute error). The grid of  $x_0$ -values was chosen to be logarithmically even spaced. The Matlab script `WKBatrest.m` solves the problem of WKB evolution of a wave-packet initially at rest with  $\langle x \rangle = \langle v \rangle = 0$ , by taking advantage of the symmetry of the problem around the origin to consider only the grid of positive values  $x_0 = 10^{i/N_F}$ , for  $i = N_S N_F, N_S N_F + 1, \dots, N_B N_F$  with integers  $N_S < N_B$  and  $N_F > 1$ . Thus, the number of  $x_0$ -values per decade is  $N_F$ , with a minimum value  $10^{N_S}$  and a maximum value  $10^{N_B}$ . The Matlab script `WKBscatter.m` solves the problem of WKB evolution of an initial wave-packet with  $\langle x \rangle, \langle v \rangle \neq 0$ . Since there is no symmetry in this problem around the center  $\langle x \rangle$  of the initial wave-packet, we used a doubled grid of points  $x_0 = \langle x \rangle + \sigma \cdot 10^{i/N_F}$ , with  $\sigma = \pm 1$  and with  $i = N_S N_F, N_S N_F + 1, \dots, N_B N_F$  as before. The two Matlab driver scripts and all functions called by them as subroutines are included as Supplementary Materials in the tar+gzipped directory “WKB codes.tar.gz”.

The integrations for the Kummer potential require numerical evaluation of the confluent hypergeometric/Kummer functions in Eqs.(S2)-(S4). The Matlab function `kummer.m` is our own modified version of `chgm.m`, which is available from the Matlab File Exchange at:

<http://www.mathworks.com/matlabcentral/fileexchange/6218-computation-of-special-functions>

The Matlab functions in this suite are a direct conversion of the corresponding Fortran programs in S. Zhang and J. Jin, “Computation of Special Functions” (Wiley, 1996), converted by the `f2matlab` open source code written by Ben Barrowes. We found that the function `chgm.m` gives inaccurate results for large negative arguments of the Kummer function, or, in practice, arguments algebraically less than  $-100$ . Our function `kummer.m` in that range uses well-known asymptotic series for large negative arguments [EB 6.13.1(2); AS 13.5.1] and, in other cases, calls `chgm.m`.

The results presented in the main text used  $N_F = 256$  with  $N_S = -15$ ,  $N_B = 1$ . Refinement studies carried out by varying the parameters  $N_F$ ,  $N_S$ ,  $N_B$  showed that these results are well converged. As a further test of accuracy, the codes evaluate the normalization of the WKB position PDF, both overall and for  $x_0$  to the right and left of  $\langle x \rangle$ . The exact results 1, .5, .5 for these normalizations were always obtained to at least a 1% accuracy and usually much more accurately.

## 2. Additional figures generated by the code

In addition to generating the plots in the main text, the codes `WKBatrest.m` and `WKBscatter.m` generate further plots that did not fit into the limited space of the paper. For example, space-time plots of the characteristic solutions  $x_t(x_0)$  for the grid of  $x_0$ -values used in the computations, plots of the phase of the WKB wave-function or classical action, etc. For more details see the accompanying text file “code\_guide.txt”, which lists and briefly describes all of the driver scripts and called functions in “WKB codes.tar.gz”. The driver scripts are all internally well-documented by programming notes, which give full details.

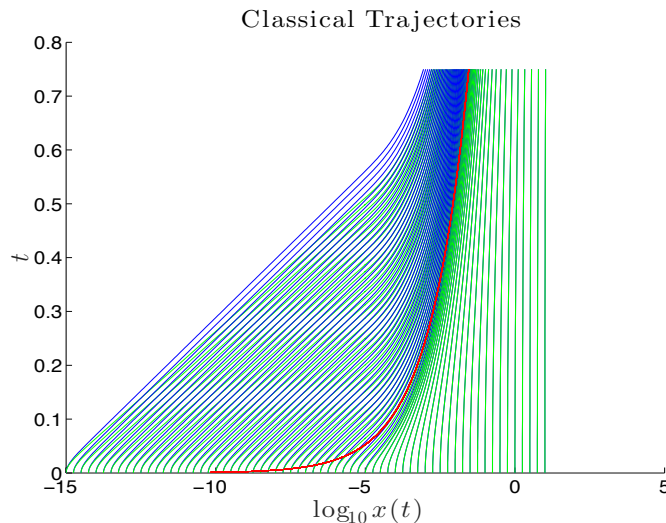

FIG. 2. Space-time plots of the classical trajectories  $x_t(x_0)$  used in the computation for the Kummer potential (blue solid) and the spliced potential (green dashed). Also shown is the extremal classical solution  $x_+(t)$  for the cusp potential (red solid). In this plot, the roughness exponent  $\alpha = 1/3$  and the UV-cutoff length  $\ell = 10^{-5}$ .

Here we include the space-time plot of the classical trajectories used in `WKBatrest.m` for the calculation of the WKB wave-function. We show only  $1/64^{th}$  of the actual number of trajectories used in that computation, for the sake of clarity of the picture. This log-linear plot illustrates very nicely the property of “forgetting” the initial data for both smooth potentials, since all solutions  $x_t(x_0)$  for choices of  $x_0$  covering more than 15 orders of magnitude in size converge rapidly to the extremal solution  $x_+(t)$  as  $t$  increases. For  $|x_0| < \ell$  the early growth is exponential, obvious as straight lines in the plot. At later times or for  $|x_0| > \ell$ , the growth becomes of explosive, Richardson type.

## 3. Bifurcation analysis for splitting-time

As discussed in the main text and in section IV.A.2 above, the bifurcation analysis to determine the splitting times is carried out by solving the combined system of Eqs.(S7),(S8) with the stated initial conditions. Let us assume an initial Gaussian wave-packet at rest at the origin with position spread  $\sigma = \ell/\mu$ . The ratio  $-J'_t(x_0)/J_t(x_0)$  is monotonically increasing in time starting from 0 for all  $x_0$  and, for a given value of  $\mu$ , the hitting time  $t_\mu(x_0)$  that it takes for  $-J'_t(x_0)/J_t(x_0)$  to reach  $x_0/\sigma^2$  (if ever) is the time at which an extremum (maximum/minimum) of the WKB position PDF  $\rho(x, t)$  is located at the corresponding point  $x = x_t(x_0)$ . The set of all of these  $(x, t)$  values (or the  $(x_0, t)$  values) constitutes the *bifurcation diagram* for the given  $\mu$  value. Furthermore, the time  $\tau$  where the graph of the non-dimensionalized function  $-J'_\tau(u_0)/J_\tau(u_0)$  first touches the line  $\mu^2 u_0$  gives the dimensionless *splitting time*  $\tau_c(\mu)$  of the WKB position PDF. For the infinitely differentiable Kummer potential, this splitting always occurs at

$u_0 = 0$  by a pitchfork bifurcation. For the spliced potential, one must minimize the non-dimensionalized hitting time  $\tau_\mu(u_0)$  over all possible  $u_0$  to obtain the splitting time  $\tau_c(\mu)$ .

Our Matlab script `bifurc.m` plots the bifurcation diagrams for a given value of  $\mu$ , both for the Kummer and for the spliced potential. The systems of ODE's in Eqs.(S7),(S8) are integrated in Matlab using the same scheme as discussed in the preceding subsection. The inclusion of the pair of eqs.(S8) requires the 3rd derivative  $V'''$ , which for the Kummer potential is obtained from `kummer.m`. The time  $\tau_\mu(u_0)$  at which  $-J'_\tau(u_0)/J_\tau(u_0)$  hits the line  $\mu^2 u_0$  for any initial  $u_0$  is obtained by using a Matlab Event function `hit.m` in the `ode113` ODE solver. Since the bifurcation for the Kummer potential is of pitchfork type at  $u_0 = u = 0$ , it suffices to consider a grid of  $u_0$ -values in a neighborhood of 0. We obtained good resolution of the bifurcation curve with 1000  $u_0$ -values logarithmically evenly spaced from  $10^{-5}$  to  $10^{-2}$  and we solved the Eqs.(S7),(S8) from  $\tau = 0$  to  $\tau = 10^4$ .

The algorithm in `bifurc.m` for the spliced potential is a bit more complicated, reflecting its more complex bifurcation structure. This is not a point of primary interest in the paper, since the spliced potential has low-order smoothness and exhibits non-generic bifurcations for small  $\mu$ . However, we briefly discuss this here in order to make the coding and output of `bifurc.m` more intelligible. Consider Eqs. (27),(28) in the main text for the limit  $-J'_\infty(u_0)/J_\infty(u_0)$  and the corresponding Fig. 5 there. For  $\mu^2 < (1+\alpha)/2$ , there are possible bifurcations occurring at  $u_0 \geq 1$ . For  $\mu \ll 1$  and  $\tau \ll 1$ , a Taylor-series analysis for the cusp potential analogous to that in Section IV.B of the main text for the Kummer potential shows that

$$-J_\tau(u_0)/J_\tau(u_0) \sim \frac{1}{2}\alpha(1-\alpha) \cdot \tau^2/u_0^{2-\alpha}, \quad \tau \ll 1.$$

Thus, the solutions of  $-J_\tau(u_0)/J_\tau(u_0) = \mu^2 u_0$  in  $\tau$  for  $\mu \ll 1$  have the form  $\tau_\mu(u_0) \sim \left(\frac{2}{\alpha(1-\alpha)}\right)^{1/2} \cdot \mu \cdot u_0^{(3-\alpha)/2}$ . For the unregulated cusp potential, this time vanishes as  $u_0 \rightarrow 0$ , so that the splitting of the wave-function is instantaneous. For the spliced model, this minimum must be taken only over  $u_0 \geq 1$ , which implies a bifurcation at  $u_0 = 1$  giving

$$\tau(\mu) \sim \left(\frac{2}{\alpha(1-\alpha)}\right)^{1/2} \cdot \mu, \quad \mu \ll 1.$$

This bifurcation is a non-generic saddle-node-type, due to the low smoothness of the potential at  $u_0 = 1$ . Note that it coexists with other (generic) saddle-node bifurcations occurring for  $0 < u_0 < 1$ . On the other hand, for  $\mu^2 > (1+\alpha)/2$  there is no possible extremum of the WKB position PDF with  $u_0 \geq 1$ , since the infinite-time limit lies there everywhere below the line  $\mu^2 u_0$ . For a value  $\mu_c \doteq 1.66$ , the line  $\mu^2 u_0$  is exactly tangent to the limit function  $-J'_\infty(u_0)/J_\infty(u_0)$  in the interval  $0 \leq u_0 < 1$ . Thus, for  $\mu > \mu_c$ , there is a subinterval of points inside the interval  $0 \leq u_0 < 1$  where  $\mu^2 u_0$  exceeds  $-J'_\infty(u_0)/J_\infty(u_0)$  and no extremum can occur. As  $\mu$  increases, the length of this subinterval grows. However, for any fixed  $\mu > \mu_c$ , there will be two separate saddle-node bifurcations with increasing  $\tau$ , one near  $u_0 = 0$  and the other near  $u_0 = 1$ .

Hence, in `bifurc.m` we must sample finely points near  $u_0 = 1$  as well as near  $u_0 = 0$  and in addition to the grid of  $u_0$ -values used for the Kummer potential, we use also a second grid with  $u_0 = 1 - v_0$ , for 1000 points  $v_0$  logarithmically evenly spaced from  $10^{-5}$  to  $10^{-10^{-2}} \simeq 1$ , and a third grid with  $u_0 = 1 + v_0$  for the same set of  $v_0$ -points. The code `bifurc.m` using these algorithms plots both bifurcation diagrams in the  $(u, \tau)$ - and  $(u_0, \tau)$ -planes, for any specified  $\mu$  parameter and for either choice of potential, Kummer or spliced.

The Matlab script `splittingTime.m` which determines the dimensionless splitting time  $\tau_c(\mu)$  uses the same basic algorithm as just described, but now a minimum over  $u_0$  must be performed for each choice of  $\mu$ . The minimization for the Kummer potential is trivial, because the bifurcation occurs at  $u_0 = 0$ . More precisely, although there is always an extremum exactly at  $u_0 = 0$ , new maxima develop infinitesimally near  $u_0 = 0$  at the time  $\tau_c(\mu)$ . Thus, in `splittingTime.m` we can simply take a very small value of  $u_0$ , close to the unit round or `eps` in Matlab, in order to determine the minimum time for the Kummer potential. In practice, we take  $u_0 = 10^{-10}$ . The computation for the spliced potential is more intensive, since a minimization of  $\tau_\mu(u_0)$  over the entire grid of  $u_0$ -values must be taken inside the loop over the desired choices of  $\mu$ , which ranges over 130 logarithmically evenly-spaced values from  $\mu = 10^{-6}$  to  $\mu = 10^7$ . Especially for large  $\mu$ -values, the grid of  $u_0$ -must be substantially better resolved than for the plotting of bifurcation diagrams in `bifurc.m` at moderate  $\mu$  values. For the results presented in Fig. 3 of the main text we used 5000 logarithmically evenly-spaced values of  $v_0$  from  $10^{-8}$  to  $10^{-10^{-9}} \simeq 1$ , and then took the union of three grids of the form  $u_0 = v_0$ ,  $u_0 = 1 - v_0$ , and  $u_0 = 1 + v_0$ . Minimization over this grid of  $u_0$ -values yielded our approximation to  $\tau_c(\mu)$  for the spliced potential.

## V. NUMERICAL SCHRÖDINGER METHODS

We numerically integrated the 1D Schrödinger equation using the solver `pySchrodinger` created by Jake Vanderplas and Andre Xuereb, publicly available at:

<https://github.com/jakevdp/pySchrodinger>

The code `schrodinger.py` permits as inputs general potentials and general normalized wave-functions as initial data. We used this code to solve the non-dimensionalized Schrödinger equations for an initial Gaussian wavepacket with  $\langle x \rangle = \langle v \rangle = 0$  in the Kummer potential centered at the origin, on a periodic domain  $[-64\pi, +64\pi]$ . The computational spacetime grid was chosen to contain  $2^M$  points, with  $M$  a positive integer, for convenience of performing FFT's. To increase speed of computations we modified the code slightly so that, rather than scipy's `fftpack`, we instead use `pyfftw`. For information on this python wrapper, see:

<https://hgomersall.github.io/pyFFTW>

We chose the time-step as  $\Delta t = \varepsilon/2R$  and the grid-spacing as approximately  $\tilde{\Delta}x = \pi\varepsilon/R$ , where we refer to  $R \geq 1$  as the “resolution.” It is essentially the number of grid points per dimensionless de Broglie wavelength  $\varepsilon$ . The actual grid spacing was then taken to be  $\Delta x = 128\pi/2^M$  with  $M = \lfloor \log_2(128\pi/\tilde{\Delta}x) \rfloor$ , the integer part. Note that  $\Delta x = \tilde{\Delta}x$  when  $R$  is a power of 2. The results of Bao et al. (2002) [ref.46] suggest that an  $R$  slightly larger than 1 should give converged results and we verified that this is true for our problem. However, the results presented in the main text were for extremely well-resolved runs with  $R = 2^7 = 128$ . In order to best study a sequence of runs which vary  $\varepsilon, \ell, \sigma$ , we wrote functions `evolve` and `save` to store and save the quantities of interest over various runs. We coupled this solver with another code, `tools.py`, which contains various analytical results stored as functions, as well as the classes `GetData` and `read_solution` which load data from multiple runs. We created a driver code `1D_Schroedinger Solver` for performing the computations as an ipython notebook. This code is also used for post-processing the data and producing all figures in the paper. All of these additions to the original code are also publicly available, at

<https://github.com/thdrivas/pySchrodinger>

## REFERENCES

- [AS] M. Abramowitz and I. Stegun, *Handbook of Mathematical Functions: with Formulas, Graphs, and Mathematical Tables*, Dover Books on Mathematics (Dover Publications, 2012). Ref.[30] in the main text.
- [EB] A. Erdélyi and H. Bateman (Bateman Manuscript Project), *Higher Transcendental Functions*, vol. 1 (Dover Publications, 2007). Ref. [31] in the main text.
- [BE] H. Bateman and A. Erdélyi (Bateman Manuscript Project), *Tables of Integral Transforms: Based, in Part, on Notes Left by Harry Bateman*, vol. 1 (McGraw-Hill, 1954). Ref. [32] in the main text.
